# Supplementary material for: FreDo: Frequency Domain-based Long-Term Time Series Forecasting
Source: arXiv:2205.12301 source file (2022-05-24)
Supplement: Supplementary file 1 [file appendix.tex]

\documentclass[aaa.tex]{subfiles}

\begin{document}

\begin{appendices}

\section{Hyperparameters} \label{app:hyper}

\section{Complex-valued Model} \label{app:complex}

\section{Hyperparmeter Search in \textsf{AverageTile}} \label{app:searchbase}

\section{Model Sizes} \label{app:modelsize}

% \section{More on Why Frequency Domain?} \label{app:whyfreq}

\end{appendices}

\end{document}
